# Supplementary material for: GEOALIGN: Geometric Rollout Curation for Robust LLM Reinforcement Learning
Source: arXiv:2606.26917 source file (2026-06-25)
Supplement: Supplementary file 1 [file more_related_works.tex]

\section{More Related Works}
\label{appendix:more_related_works}

\zhenqing{TBD: Add more citations or remove this sec?}

\subsection{Reward-Centric Robust RL}
% % Controlling Magnitude, Ignoring Direction; They conflate reward magnitude with improvement validity.

Most robust RL approaches for LLM alignment operate under an implicit but critical assumption: that scalar reward values reliably encode the \textit{direction} of desirable policy improvement. Under this view, instability arises primarily from \textit{over-optimization} or \textit{noisy magnitudes}, and can be mitigated by reshaping rewards~\cite{par}, clipping extremes~\cite{yang2024regularizing}, or adaptively scaling learning rates based on prompt-level uncertainty~\cite{seedgrpo,li2025limr}. While effective at stabilizing training, these methods treat rewards as unstructured scalars and apply uniform or uncertainty-modulated weighting across all high-reward samples. They do not distinguish between rollouts that induce consistent representational shifts versus those that pull the policy in orthogonal or adversarial directions—even when both receive similar rewards. In essence, they conflate reward magnitude with improvement validity.

\subsection{Rollout Selection and Filtering}
%Heuristics Without Geometric Awareness
Recognizing that not all high-reward rollouts are equally informative, recent work proposes to filter or reweight samples based on reward variance~\cite{pods}, score distribution~\cite{zhang2024policy}, or semantic entropy~\cite{seedgrpo}. For instance, PODS maximizes intra-rollout reward variance to prioritize ``informative'' samples~\cite{pods}, while PF-PPO avoids mid-score regions prone to reward model errors~\cite{zhang2024policy}. However, these strategies remain heuristic and reward-statistics-driven: they lack a principled mechanism to assess whether a rollout’s induced update aligns with the global trajectory of alignment. Consequently, they may retain rollouts that achieve high rewards through spurious shortcuts—precisely the source of directional inconsistency we aim to address.
(Optional, In our experiments (Sec. X), we observe that high-variance or high-entropy rollouts often exhibit large angular deviation from the consensus direction.)

\subsection{Gradient-Based Attribution}
%Direction-Aware but Inefficient; 
A few recent methods attempt to directly inspect update directions by computing per-sample gradients or influence scores~\cite{hu2025snapshot,dai2025dataefficacylanguagemodel}. Snapshot of Influence~\cite{hu2025snapshot}, for example, identifies harmful samples by measuring their impact on policy parameters along the optimization path. While conceptually aligned with our goal of detecting conflicting updates, these approaches require expensive second-order computations or additional backward passes, making them impractical for large-scale online RL where thousands of rollouts are generated per step. Moreover, they operate in parameter space rather than representation space, missing the opportunity to leverage the rich geometric structure of LLM latents.
In contrast, GeoAlign operates in the representation space—where alignment signals are more structured—and estimates directional consistency using only forward-pass features, enabling real-time deployment.

\subsection{Geometric Perspectives in Representation Learning}
While geometric reasoning has been extensively explored in self-supervised learning—e.g., via alignment/uniformity tradeoffs~\cite{wang2020understanding}, manifold clustering~\cite{arora2019theoretical}, or neural collapse~\cite{papyan2020prevalence}—its application to reinforcement learning remains nascent. Our work bridges this gap by treating policy improvement as a \textit{directional alignment problem} in latent space, where the goal is not just to maximize reward, but to ensure that reward-induced transitions cohere with an evolving geometric consensus.
% }
