# Supplementary material for: GEOALIGN: Geometric Rollout Curation for Robust LLM Reinforcement Learning
Source: arXiv:2606.26917 source file (2026-06-25)
Supplement: Supplementary file 2 [file content.tex]

\section*{Appendix}
\label{sec:appendix}

\DoToC
